# Supplementary material for: Correcting for Interference in Experiments: A Case Study at Douyin
Source: arXiv:2305.02542 source file (2023-05-04)
Supplement: Supplementary file 1 [file appendix.tex]

\section{}

\section{Variance of DQ Under the Sharp Null}

关于Delta Method的理论验证
考虑在用户i上，主播l对主播t的DQ贡献（此处我们假设non-dependent action，方法与结论可以推广到dependent情况）：

$$ x_{t\rightarrow l}^{i} := \left(\frac{1(a_t=1)1(a_{l}=1)}{p_1^2}r_{i,l} - \frac{1(a_{l}=1)}{p_1}r_{i,l}\right) - \left(\frac{1(a_t=0)1(a_{l}=0)}{p_0^2}r_{i,l} - \frac{1(a_{l}=0)}{p_0}r_{i,l}\right)$$
$$ x_{t\rightarrow t}^{i} := \frac{1(a_t=1)}{p_1}r_{i,t} - \frac{1(a_t=0)}{p_0}r_{i,t}$$

让我们对用户和主播进行加总
$$ x_{t\rightarrow l} = \sum_{i \in [N]} x_{t\rightarrow l}^{i}, x_{t} = \sum_{l} x_{t\rightarrow l}$$
注意DQ就是
$$  \hat{\tau} =\frac{1}{N}\sum_{t \in [M]} x_{t}$$
我们的目标是计算AA情况下DQ的方差，这种情况下
$$  Var[\hat{\tau}]=E[\hat{\tau}^2]=\frac{1}{N^2}E\left[\left(\sum_{t} x_{t}\right)^2\right] = \frac{1}{N^2}E\left[\sum_{t,l,i,j} x_{t\rightarrow l}x_{i\rightarrow j}\right]$$
引理1：对于任意的$$ t\in[M], l\in[M]/\{t\}, a\in \{0,1,2\}$$, 我们都有$$ E[x_{t\rightarrow l}^{i} | a_{l}=a] = 0$$
引理2：对于任意的$$ t\in[M], l\in[M]$$, 我们都有$$ E[x_{t\rightarrow l}^{i}] = 0$$
证明：直接验证即可。

接下来对于$$E\left[x_{t\rightarrow l}x_{i\rightarrow j}\right]$$ (t不等于i时)，我们考虑几种情况

1.  $$t,l,i,j$$互不相同：这种情况下$$x_{t\rightarrow l} 和x_{i\rightarrow j}$$互相独立，所以
$$E\left[x_{t\rightarrow l}x_{i\rightarrow j}\right] = E[x_{t\rightarrow l}]E[x_{i\rightarrow j}] = 0$$
2. $$l=j$$时，此时对于任意的$$a\in \{0,1,2\}$$, 我们有
$$E\left[x_{t\rightarrow l}x_{i\rightarrow l} | a_{l}=a\right] = E[x_{t\rightarrow l} | a_{l}=a]E[x_{i\rightarrow l}|a_{l}=a] = 0$$
注意这里我们用到了condition on a_{l}以后，$$x_{t\rightarrow l} 和x_{i\rightarrow l}$$就独立了（因为a_{t}和a_{l}独立）

所以再用全概率公式
$$E\left[x_{t\rightarrow l}x_{i\rightarrow l}\right] = \sum_{a}E\left[x_{t\rightarrow l}x_{i\rightarrow l} | a_{l}=a\right] p(a_{l}=a) = 0$$
3. $$l=i~,~j\neq t $$时，对于任意的$$a\in \{0,1,2\}$$, 我们再次有
$$E\left[x_{t\rightarrow i}x_{i\rightarrow j} | a_{i}=a\right] = E[x_{t\rightarrow i} | a_{i}=a]E[x_{i\rightarrow j}|a_{i}=a] = 0$$
这里用到了$$ E[x_{t\rightarrow i} | a_{i}=a] = 0$$
4. 最后只剩下一种情况 $$E\left[x_{t\rightarrow i}x_{i\rightarrow t}\right]$$，这种情况不能抵消。通过计算可以得出：
$$E\left[x_{t\rightarrow i}x_{i\rightarrow t}\right] = \left(\frac{(1-p_1)^2}{p_1^2} + \frac{(1-p_0)^2}{p_0^2} - 2\right) r_{tl}r_{lt} = \frac{1-2p_1}{p_1^2} + \frac{1-2p_0}{p_0^2}$$

所以
$$  E\left[\sum_{t,l,i,j} x_{t\rightarrow l}x_{i\rightarrow j}\right] = \sum_{t}E\left[x_{t}^2\right] + E\left[\sum_{t\neq i}x_{t\rightarrow i}x_{i\rightarrow t}\right]$$
在我们的仿真中：
$$  E\left[\sum_{t\neq i}x_{t\rightarrow i}x_{i\rightarrow t}\right]$$对结果的贡献非常小（在主播基本同质的情况下，可以进行理论说明），所以我们用$$  E\left[\sum_{t,l,i,j} x_{t\rightarrow l}x_{i\rightarrow j}\right] \approx \sum_{t}E\left[x_{t}^2\right]$$进行了近似。【如果要进行精确计算，也只需要O(M^2)的时间复杂度，M是主播数】

\subsection{Taylor series expansions for total reward MDPs}

Taylor expansions for several {\it total reward} MDP formulations follow immediately from this bound. In particular, consider Markov chains $P$ with one or more absorbing states, and let $\tilde{P}$ be the submatrix corresponding to all transient states. Then, we have that $\|\tilde{P}\| < 1$, and as result
\begin{equation*}
J_{\pi} = \rho_{\rm init}(\sum_{t=0}^{\infty} \tilde{P}^{t})r_{\pi}= \rho_{\rm init}(I - \tilde{P})^{-1} r_{\pi}
\end{equation*}

\cref{th:taylor-fundamental} then immediately implies the Taylor series expansion for $J_\pi$:

\begin{corollary}
  \label{co:taylor-absorbing}
Let $\pi, \pi'$ be policies inducing transition kernels $P,P' \in \mathbb{R}^{n \times n}$, where both kernels have a single absorbing state. Let $\tilde{P}, \tilde{P}^{\prime} \in \mathbb{R}^{(n-1)\times(n-1)}$ be the submatrices corresponding to the transient states. Then,
\begin{equation*}
J_{\pi} = \rho_{\rm init}^\top(I-\tilde{P})^{-1}\left(\sum_{k=1}^{K} \left[(\tilde{P}^{\prime}  - \tilde{P}) (I - \tilde{P}^{\prime})^{-1}\right]^{K} \right) r_{\pi} + \rho_{\rm init}^\top(I - \tilde{P}')^{-1} \left[(\tilde{P}' - \tilde{P}) (I - \tilde{P})^{-1} \right]^{K+1} r_{\pi}
\end{equation*}
\end{corollary}

Total reward in fixed-horizon Markov chains follows as a special case of this result, by augmenting the state space with a time index, and adding a deterministic transition to an absorbing state at the end of the horizon.

%   \label{co:taylor-discounted}
% Let $\pi, \pi'$ be policies inducing transition kernels $P,P' \in \mathbb{R}^{n \times n}$, and let $\gamma < 1$. Then, we have that
%   \begin{equation*}
% J_{\pi'}^{\gamma} = \rho_{\rm init}^\top(I-\gamma P)^{-1}\left(\sum_{k=0}^{K}\gamma^{K}\left[(P^{\prime}  - P) (I - \gamma P^{\prime})^{-1}\right]^{K} \right) r_{\pi'} + \gamma^{K+1}\rho_{\rm init}^\top(I - \gamma P')^{-1} \left[(P' - P) (I - \gamma P)^{-1} \right]^{K+1} r_{\pi'}
% \end{equation*}
% \end{corollary}

\subsection{Unifying total reward and average reward expansions}

In the derivation of the average-reward DQ estimator in \cref{chapter:markovian-interference}, we relied essentially on the following perturbation bound on the stationary distributions of ergodic Markov chains:
\begin{lemma}
  \label{lem:perturbation-average-reward}
  Let $P, P' \in \mathbb{R}^{n \times n}$ be irreducible stochastic matrices with stationary distributions $\rho, \rho' \in \mathbb{R}^{n}$. Then,
  \begin{equation*}
(\rho')^\top = \rho^\top + (\rho')^\top (P' - P) (I - P)^{\#}
  \end{equation*}
\end{lemma}

In this section, we will provide a mostly self-contained proof of this lemma as the limit of an appropriate normalization of the Taylor expansion for the discounted reward.

\begin{proof}
  Let $\rho_{0} \in \mathbb{R}^{n}$  be any distribution (more precisely, any vector such that $\rho_0^\top {\bf 1} = 1$. As before, \cref{lem:perturbation-fundamental} immediately yields
  \begin{equation}
    \label{eq:perturbation-discounted}
(1 - \gamma) (I - \gamma P')^{-1} = (1 - \gamma) (I- \gamma P)^{-1}  + (1 -\gamma) \gamma (I - \gamma P')^{-1}(P' - P) (I - \gamma P)^{-1}
  \end{equation}
The proof will procced by taking the limit as $\gamma \to 1$ of the expression above. First, we show that
  \begin{equation}
    \label{eq:perturbation-limit-1}
\lim_{\gamma \to 1} (1 - \gamma) (I - \gamma P)^{-1} = 1 \rho^\top
\end{equation}
To see this, we can use the Jordan form of $I - \gamma P$:
\begin{equation*}
  I - \gamma P = W \begin{bmatrix} 1 - \gamma & 0 \\ 0 & I - \gamma Q \end{bmatrix} W^{-1}
\end{equation*}
and it then immediately follows that
\begin{align*}
  (1 - \gamma)(I - \gamma P)^{-1}
  &= W \begin{bmatrix} 1 & 0 \\ 0 & \lim_{\gamma \to 1}(1 - \gamma) (I - \gamma Q)^{-1} \end{bmatrix} W^{-1} \\
  &= W \begin{bmatrix} 1 & 0 \\ 0 & 0 \end{bmatrix} W^{-1} \\
  &= {\bf 1} \rho^\top
\end{align*}
Next, we show that
\begin{equation}
    \label{eq:perturbation-limit-2}
    \lim_{\gamma \to 1} \gamma (P' - P)(I - \gamma P)^{-1} = (P' - P) (I - P)^{\#}
\end{equation}
To see this, we first have that
\begin{align*}
  \gamma (P' - P) ( I - \gamma P ) ^{-1} = \gamma (P' - P) (( I - \gamma P ) ^{-1} - 1 \rho^\top)
\end{align*}
Next, again looking at the Jordan form of $(I - \gamma P)^{-1}$,  we have that
\begin{align*}
  \lim_{\gamma \to 1} \gamma ((I - \gamma P)^{-1}  - 1 \rho^\top)
  &= W \begin{bmatrix} 0 & 0 \\ 0 & \lim_{\gamma \to 1} \gamma (I - \gamma Q)^{-1} \end{bmatrix} W^{-1} \\
  &= W \begin{bmatrix} 0 & 0 \\ 0 & (I - Q)^{-1} \end{bmatrix} W^{-1} \\
  &= (I - P)^{\#}
\end{align*}
Taking these facts, we take the limit as $\gamma \to 1$ of \cref{eq:perturbation-discounted}, yielding
  \begin{align*}
    \lim_{\gamma \to 1}(1 - \gamma) (I - \gamma P')^{-1}
    &= \lim_{\gamma \to 1} \left[ (1 - \gamma) (I- \gamma P)^{-1}  + (1 -\gamma) \gamma (I - \gamma P')^{-1}(P' - P) (I - \gamma P)^{-1} \right] \\
    1 (\rho')^\top &= 1 \rho^\top  +  \lim_{\gamma \to 1} \gamma 1 (\rho')^\top (P' - P) (I - \gamma P)^{-1}  \\
     &= 1 \rho^\top  +  1 \rho^\top (P' - P) (I - P)^{\#}  \\
  \end{align*}
Pre-multiplying by $\rho^\top$ (or any distribution $v^\top$  such that $v^\top {\bf 1} = 1$) yields the result.
\end{proof}

%%% Local Variables:
%%% mode: latex
%%% TeX-master: "main.tex"
%%% End:
